# Supplementary material for: A Duality Based 2-Approximation Algorithm for Maximum Agreement Forest
Source: arXiv:1811.05916 source file (2018-11-14)
Supplement: Supplementary file 1 [file appendix.tex]

%
%
%
%
%
%
%
%
%
%
%
%
%
%
%
%
%
%

%
%


%
%
%

%
%
%
%

%
%
%
%
%
%
